# Supplementary material for: Acoustic phonon-restricted four-phonon interactions: Impact on thermal and thermoelectric transport in monolayer h-NbN
Source: arXiv:2505.12520 source file (2025-10-22)
Supplement: Supplementary file 1 [file h-NbN-SM.pdf]

# Thermal and thermoelectric transport in monolayer h-NbN: Roles of four-phonon scattering and tensile strain

Himanshu Murari,<sup>1</sup> Subhradip Ghosh,<sup>1</sup> Mukul Kabir,<sup>2</sup> and Ashis Kundu<sup>2</sup>

<sup>1</sup>Department of Physics, Indian Institute of Technology Guwahati, Guwahati 781039, Assam, India

<sup>2</sup>Department of Physics, Indian Institute of Science Education and Research (IISER) Pune, P.O. 411008, India

(Dated: 18th May 2025)

## I. SUPPLEMENTARY RESULTS

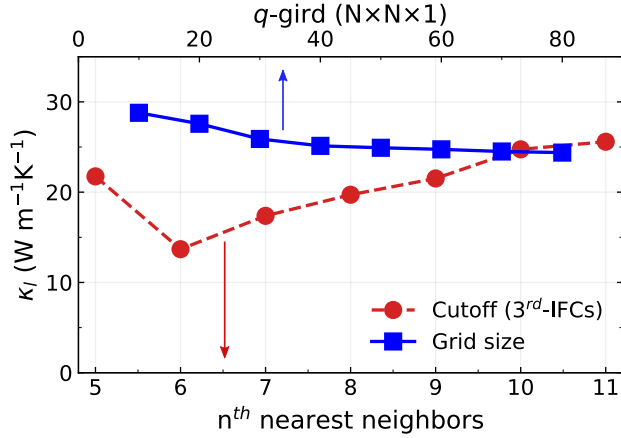

Figure S1: Calculated lattice thermal conductivity ( $\kappa_l$ ) at 300 K as a function of the  $n^{\text{th}}$  nearest neighbor cutoff for third-order interatomic force constants (IFCs) and the  $q$ -grid size ( $N \times N \times 1$ ). Convergence is achieved at the  $10^{\text{th}}$  nearest neighbor cutoff and a  $60 \times 60 \times 1$   $q$ -grid.

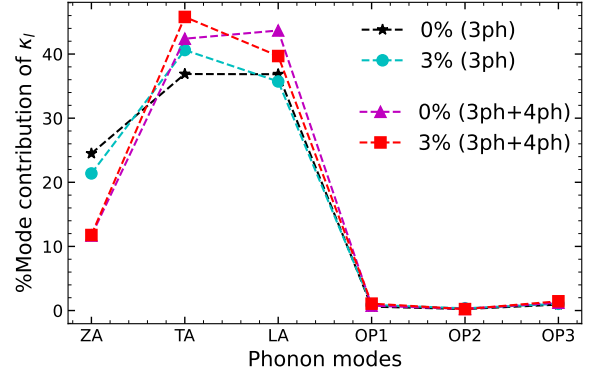

Figure S3: The percentage contribution of phonon modes to the lattice thermal conductivity ( $\kappa_l$ ) reveals that acoustic modes dominate regardless of the scattering order and applied strain. ZA, TA, and LA correspond to the three acoustic modes, while OP1, OP2, and OP3 denote the optical modes.

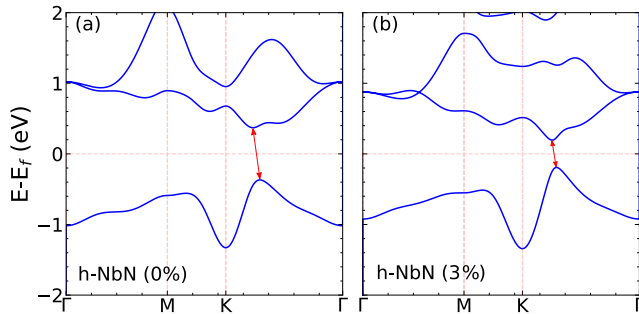

Figure S2: The electronic band structure reveals an indirect band gap along the  $K - \Gamma$  path for both unstrained ( $\epsilon = 0\%$ ) and strained ( $\epsilon = 3\%$ ) h-NbN. The band gap decreases under strain. The Fermi level is set to 0 eV.

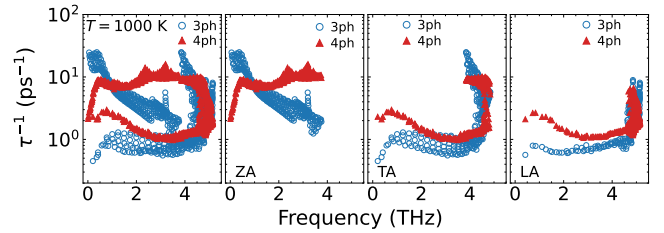

Figure S4: Comparison of three- and four-phonon scattering reveals that four-phonon processes increase more rapidly with temperature than three-phonon processes. Mode-resolved contributions further clarify this trend, showing that four-phonon scattering in the TA and LA modes surpasses their three-phonon counterparts.

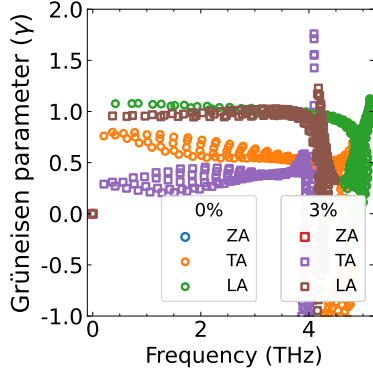

Figure S5: The Grüneisen parameter ( $\gamma$ ) reflects the anharmonicity of the system and is primarily dominated by the ZA mode, which is significantly suppressed under tensile strain (as shown in the main paper). Here, we highlight the suppression of  $\gamma$  for TA and LA modes under strain.

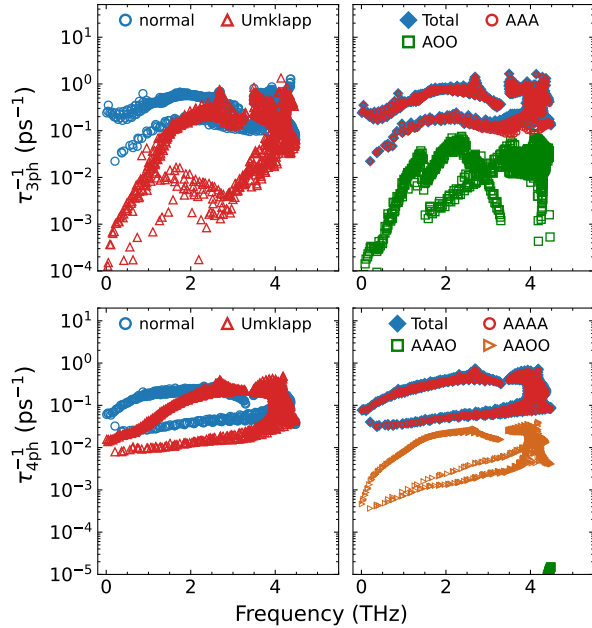

Figure S6: (a) Three-phonon (3ph) (b) four-phonon (4ph) scattering rates are presented. At 300 K, both three-phonon and four-phonon scattering in monolayer h-NbN are also predominantly governed by normal processes rather than Umklapp scattering under tensile strain 3%. Moreover, phonon scattering is primarily driven by all-acoustic processes, specifically the AAA and AAAA channels.

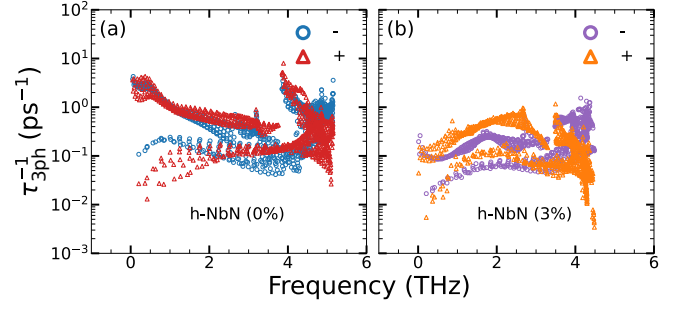

Figure S7: At 300 K, three-phonon scattering in h-NbN is dominated by absorption (+) processes rather than decay (-) events, under both unstrained and strained conditions.

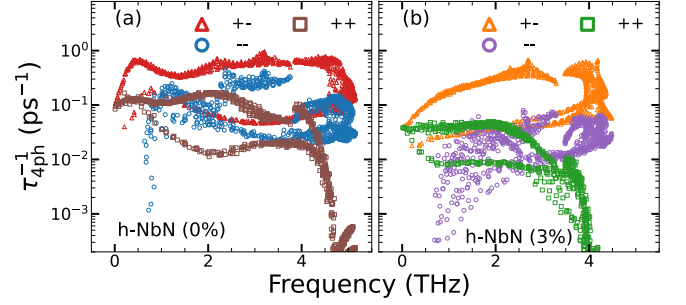

Figure S8: At 300 K, four-phonon scattering in h-NbN is predominantly governed by redistribution (+-) events over splitting (--) and recombination (++) events, for both unstrained and strained conditions.

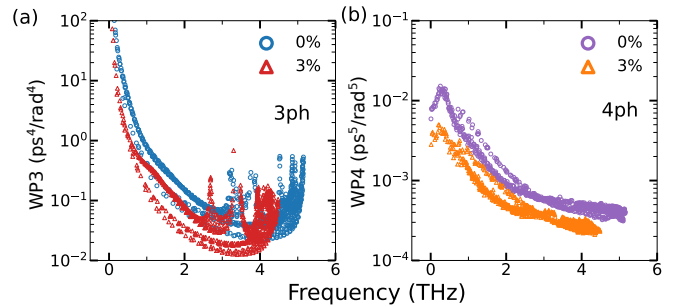

Figure S9: The weighted phase space for both three- and four-phonon processes decreases under strain, leading to reduced phonon scattering and an increase in lattice thermal conductivity at 300 K.

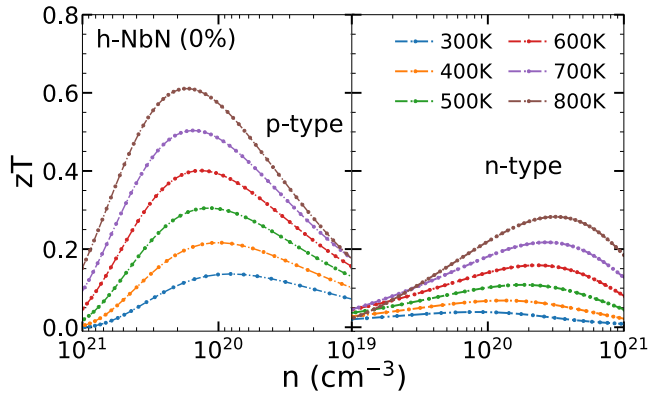

Figure S10: Variation of the figure of merit ( $zT$ ) with carrier concentration ( $n$ ) for both p- and n-type at different temperatures reveals the optimal doping levels required for enhanced thermoelectric performance. The  $zT$  values are evaluated using the lattice thermal conductivity considering both three- and four-phonon scattering ( $\kappa_l^{3ph+4ph}$ ).

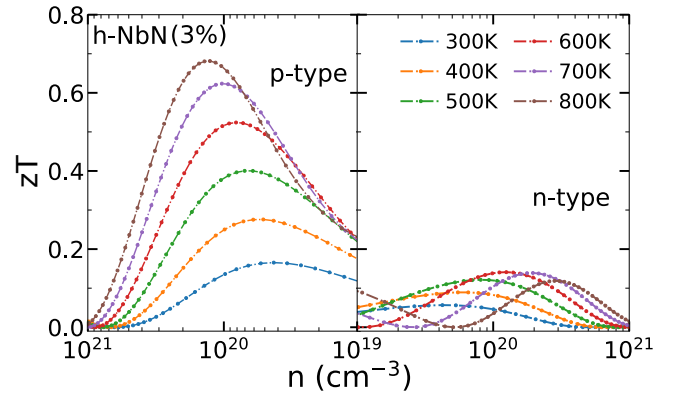

Figure S11: Variation of the figure of merit ( $zT$ ) with carrier concentration ( $n$ ) for both p- and n-type at different temperatures reveals the optimal doping levels required for enhanced thermoelectric performance. The  $zT$  values are evaluated using the lattice thermal conductivity considering both three- and four-phonon scattering ( $\kappa_l^{3ph+4ph}$ ). These results correspond to the case under 3% tensile strain.
